# Supplementary material for: Floquet-engineering the exceptional points in parity-time-symmetric magnonics
Source: arXiv:2310.09300 source file (2023-10-08)
Supplement: Supplementary file 1 [file period-PT_supp.pdf]

# Supplementary Information: Floquet-engineering the exceptional points in parity-time-symmetric magnonics

Xi-guang Wang[1], Lu-lu Zeng[1], Guang-hua Guo[1], Jamal Berakdar[2*]

[1] *School of Physics and Electronics,*

*Central South University, Changsha 410083, China*

[2] *Institut für Physik, Martin-Luther Universität*

*Halle-Wittenberg, 06099 Halle/Saale, Germany*

[*] *email: jamal.berakdar@physik.uni-halle.de*

(Dated: October 8, 2023)

## I. INFLUENCE OF MAGNETIC DAMPING

In this section, we provide more details on the effect of the magnetic damping on the Floquet PT-symmetry. We used $\alpha = 0.004$ in the main text but $\alpha$ ca be even two orders of magnitude smaller for Yttrium–Iron–Garnet (YIG). Using Eq. (6) in the main text, we include a small damping $\alpha = 2 \times 10^{-5}$. Here, the quasienergies $\epsilon_\pm$ are quite similar to the case with negligible damping of the main text, and one can still clearly identify the same quasienergy EPs and PT-symmetry broken phases (Fig. S1). With larger damping $\alpha = 0.004$ (used in the main text), in the PT-symmetry broken phase we find small gaps are generated between the real parts, and two $\mathrm{Re}[\epsilon_\pm]$ coalesce only at the center, and two imaginary parts $\mathrm{Im}[\epsilon_\pm]$ are still obviously more separated there. Besides, the damping brings a finite $\mathrm{Im}[\epsilon_\pm]$ outside the PT-symmetry broken phases. These larger finite damping induced features make the quasienergy EPs not as clear as the case with very small damping. However, one can still identify the quasi-EPs (or adjacent regions) and PT-symmetry broken phase from the region with more separated $\mathrm{Im}[\epsilon_\pm]$. Moreover, in the Floquet theorem these quasienergies are obtained from $V_\pm = e^{-i\epsilon_\pm T}$, indicating the real components of quasienergies $\epsilon_\pm T$ have the period of $2\pi$. I.e., using $\epsilon_\pm = \epsilon_\pm \pm \frac{2n\pi}{T} = \epsilon_\pm \pm n\omega_\mathrm{F}$, the physical meaning remains unchanged, where the integer $n = 0, \pm 1, ....$ With this feature, in Fig. S1, we rescaled $\mathrm{Re}[\epsilon_\pm]$ between $-\frac{\omega_\mathrm{F}}{2}$ and $\frac{\omega_\mathrm{F}}{2}$.

## II. DETAILS OF MAGNETIZATION DYNAMICS

In this section, we provide more details of magnetization dynamics under constant and time period SOT term $\omega_\mathrm{J}$. The magnetization dynamics are obtained from micromagnetic simulations based on the Landau-Lifshitz-Gilbert(LLG) equation, and to initially excite the magnetization oscillation in a wide-frequency range, we adopt a sinc pulse $h(t) = h_\mathrm{a}\mathbf{z}\sin(\omega_\mathrm{F}t)/(\omega_\mathrm{F}t)$ with amplitude $h_\mathrm{a} = 1\times 10^5$ A/m and frequency range $\omega_\mathrm{F}/(2\pi) = f_\mathrm{H} = 50$ GHz (applied locally to the region $x = 0$). For the constant SOT, the system becomes unstable $\omega_\mathrm{J} > \kappa$. As proved by Fig. S2, the magnetization oscillations ($x$ and $z$ components) perpendicular to the stable magnetization (along $+y$ direction) is quickly amplified at the beginning, and soon the amplified oscillation siwthced the magnetization to $-y$ direction. This effect is similar to the magnetization reversal driven by spin-transfer torque, where the

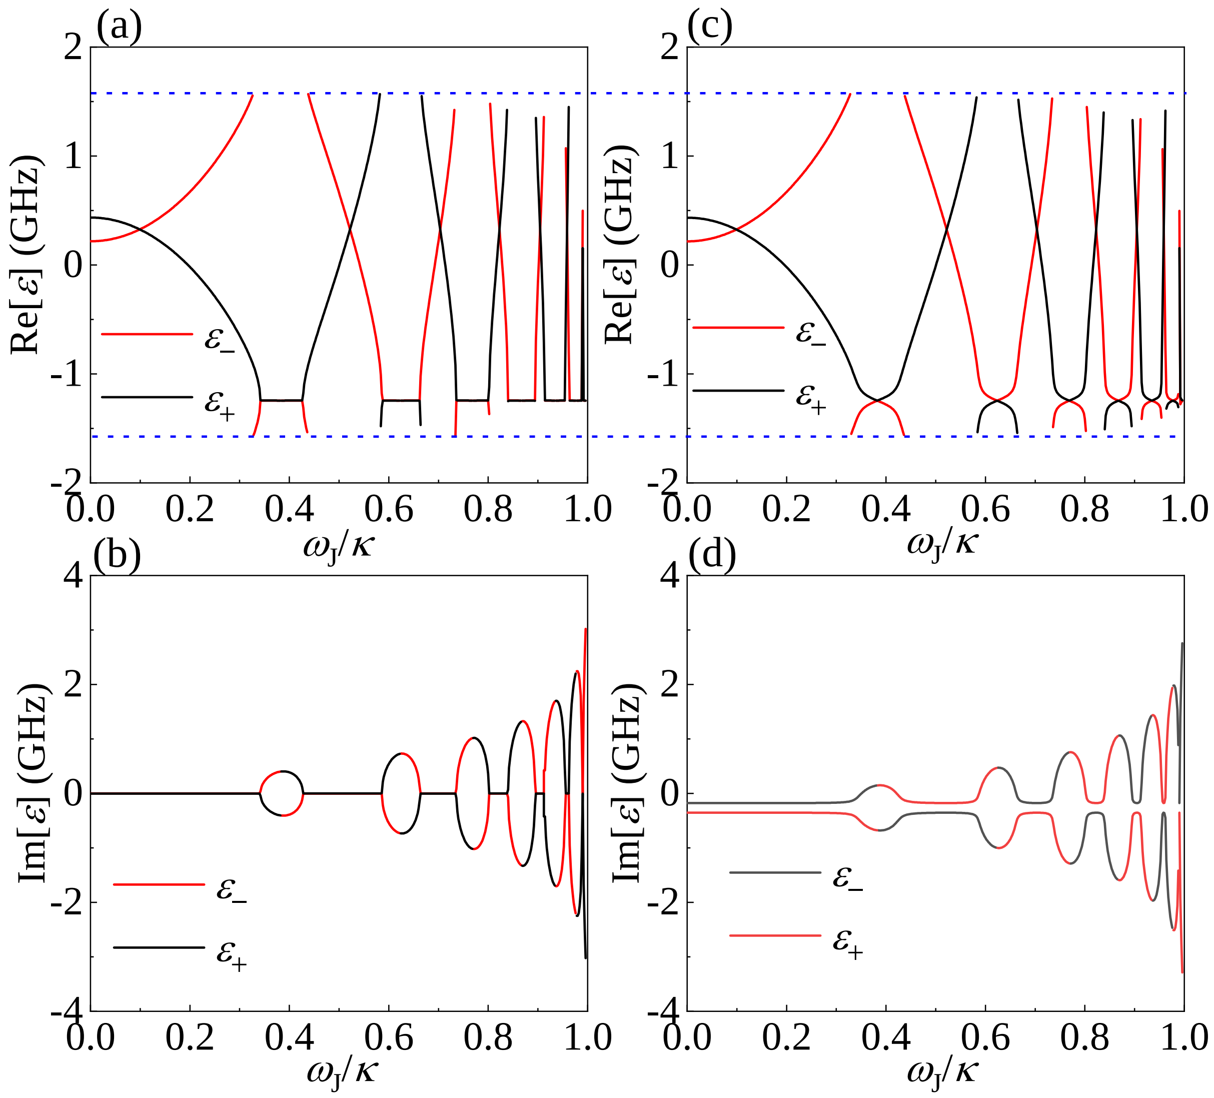


FIG. S1. Under (a-b) $\alpha = 2 \times 10^{-5}$ or (c-d) $\alpha = 0.004$ same to the main text, real and (b) imaginary parts of Floquet quasienergies $\epsilon_{\pm}$ (calculated from Eq. (6) in the main text).

spin accumulation antiparallel to the magnetic moment causes the imaginary part of the magnetic moment's intrinsic frequency to change from negative to positive, leading to an amplification of magnetic moment oscillation and eventually causing magnetization reversal [1, 2]. As the spin-wave excited from the left end propagate toward the right side, the spin-wave amplification and hence magnetization reversal also starts from the left end, see the magnetization profiles at different time points in Fig. S3. If for $\omega_{\rm J} \leq \kappa$, the system keeps stable, and the excited spin-wave is finally damped, as proved by the magnetization oscillation in Fig. S4.

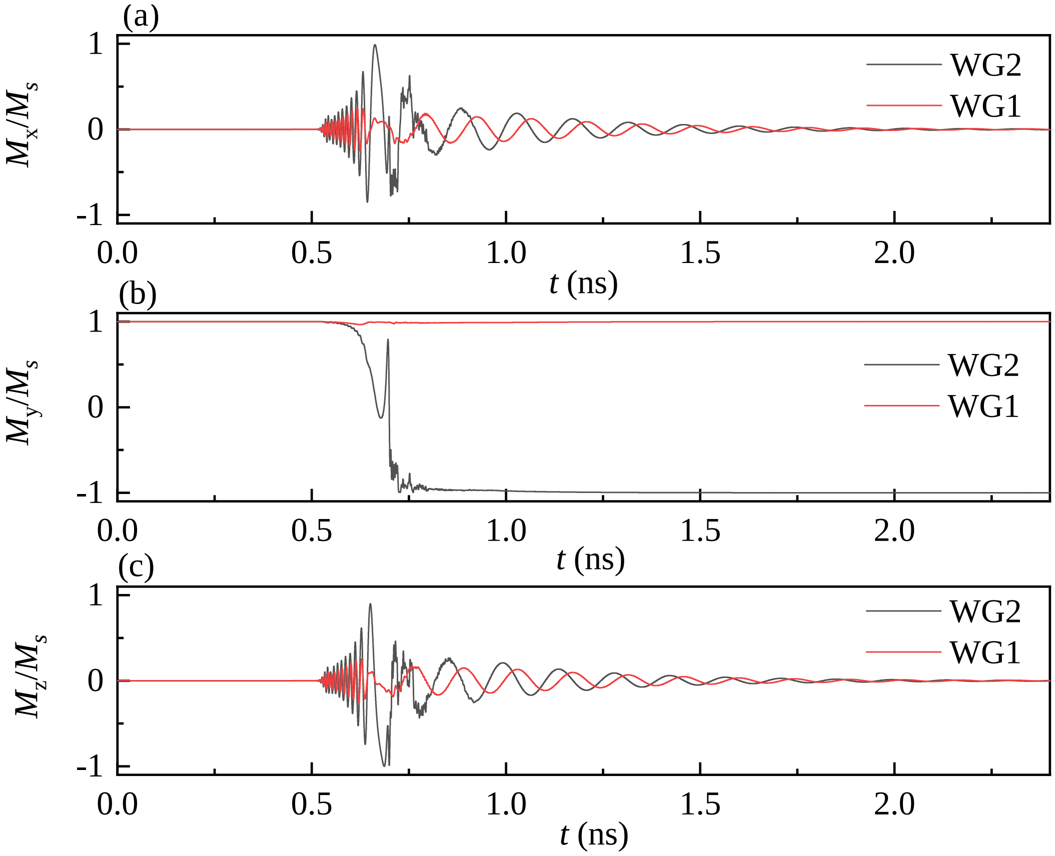


FIG. S2. For constant SOT term $\omega_J = 1.1\kappa$, time-dependent (a) $M_x$, (b) $M_y$ and (c) $M_z$ at $x = 2000$ nm in WG1 and WG2. We excite spin waves over a wide range by applying a sinc pulse $h(t) = h_a \mathbf{z} \sin(\omega_F t)/(\omega_F t)$ with amplitude $h_a = 1 \times 10^5$ A/m and frequency range $\omega_F/(2\pi) = f_H = 50$ GHz, applied locally to the region $x = 0$. The results are obtained from micromagnetic simulation based on the LLG equation.

Besides, in the main text, for the time periodic SOT, we mainly focus on the magnetization auto-oscillation in the instability range. We note, outside the instability range, for example with the periodic SOT amplitude $\omega_J/\kappa = 0.35$ and $\omega_J/\kappa = 0.43$, the excited spin-wave is damped without amplification, as proved by Fig. S5.

## III. MAGNONICS WITH SPATIALLY-PERIODIC GAIN/LOSS MECHANISM

In the main text, the periodic varying SOT is realized in the time domain. In this section, we analyze a spatially-periodic SOT, meaning gain/loss grating as shown in Figs. S6. As the spin-wave also experiences periodically varying gain and loss during the propagation,

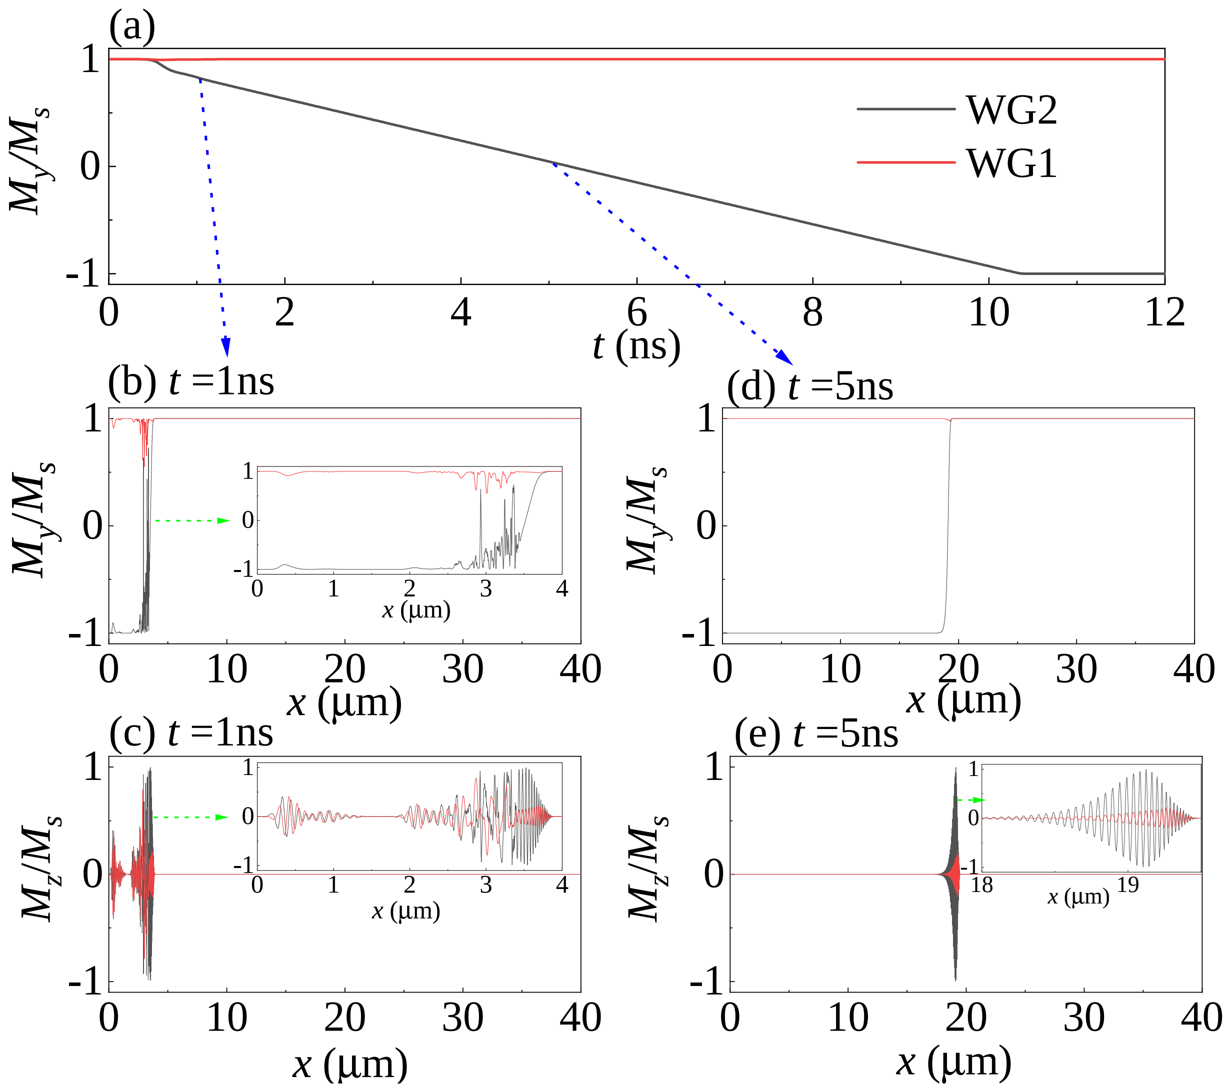


FIG. S3. For constant SOT term $\omega_{\rm J} = 1.1\kappa$, (a) time-dependent averaged $M_{\rm y}$ in WG1 and WG2. At the time point (b-c) $t = 1$ ns and (d-e) $t = 5$ ns, the spatial profile of $M_{\rm y}$ and $M_{\rm z}$ along the $x$ axis. The results are obtained from micromagnetic simulation based on the LLG equation. The lenghth of WG1 and WG2 is $40\mu$m. The insets enlarge the variations in narrow ranges.

similar effects are to be expected, including lower EPs or auto-oscillation in the broken PT-symmetry phase above EP.

Via periodic nanostructuring, adjacent Pt stripes (each with width $L$) separated with a distance $L$ carry opposite-sign charge current densities along the $y$-axis. WG1 and WG2 are both magnetized along $+x$ direction. In such setting, the SOTs are $\mathbf{T}_{1(2)} = \gamma c_{\rm J}(x)\mathbf{m}_{1(2)} \times (\pm\mathbf{x}) \times \mathbf{m}_1(2)$. Here, the SOT strength coefficient $c_{\rm J} = \frac{S\theta_{\rm SH}\hbar J_{\rm Pt}(x)}{2\mu_0 e t_{\rm p} M_{\rm s}}$ is proportional to the

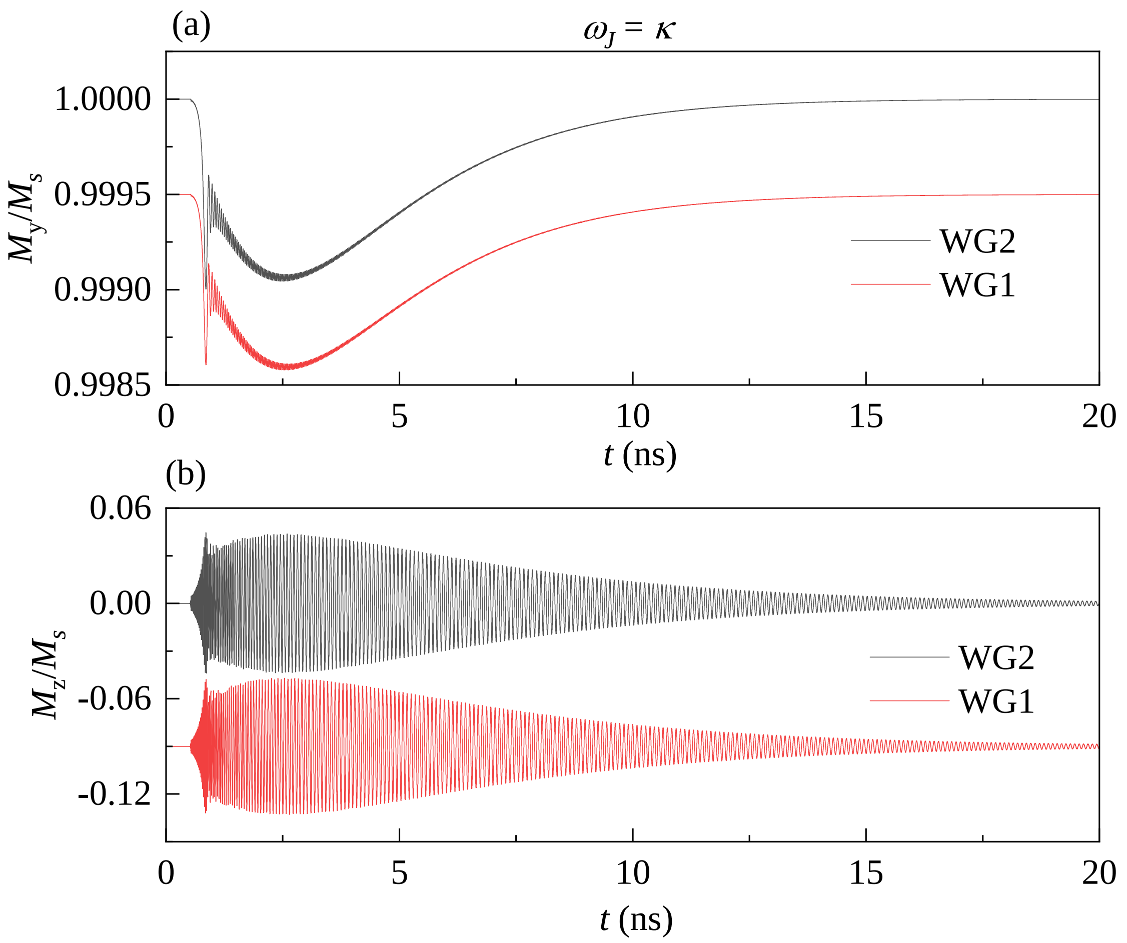


FIG. S4. For constant SOT term $\omega_{\rm J} = \kappa$, time-dependent (a) $M_{\rm y}$ and (b) $M_{\rm z}$ at $x = 2000$ nm in WG1 and WG2 obtained from micromagnetic simulation based on the LLG equation. We excite spin waves over a wide range by applying a sinc pulse $h(t) = h_{\rm a}\mathbf{z}\sin(\omega_{\rm F}t)/(\omega_{\rm F}t)$ with amplitude $h_{\rm a} = 1 \times 10^5$ A/m and frequency range $f_{\rm H} = 50$ GHz, applied locally to the region $x = 0$. The red curves (WG1) are in the same range with WG2 curves, which are intentionally offset for clarity.

charge current density $J_{\rm Pt}(x)$ (its spatial profile see Fig. S6(b)), the spin-Hall angle $\theta_{\rm SH}$ of the spacer, and the WG/spacer interface transparency $S$. Following, we define the periodic SOT term $\omega_{\rm J}(x) = \frac{\gamma c_{\rm J}(x)}{1+\alpha^2}$, and its maximum amplitude is $\omega_{\rm J0}$. In addition, in the range without Pt stripes, the interlayer exchange coupling is suppressed, resulting in periodic varying coupling strength $q(x)$. Following the same procedure adopted above and using the Bloch theorem, we obtain a solution to the magnon dynamics equation (similar to Eq. (2) in the main text) in the form of Bloch waves $\psi_{\rm p}(x) = e^{ikx}u_{\rm p}(x)$, and the function $u_{\rm p}(x) = u_{\rm p}(x + \frac{\pi}{k_{\rm J}})$ has the periodicity of the SOT term. Inserting this Bloch ansatz into the equations of motion,

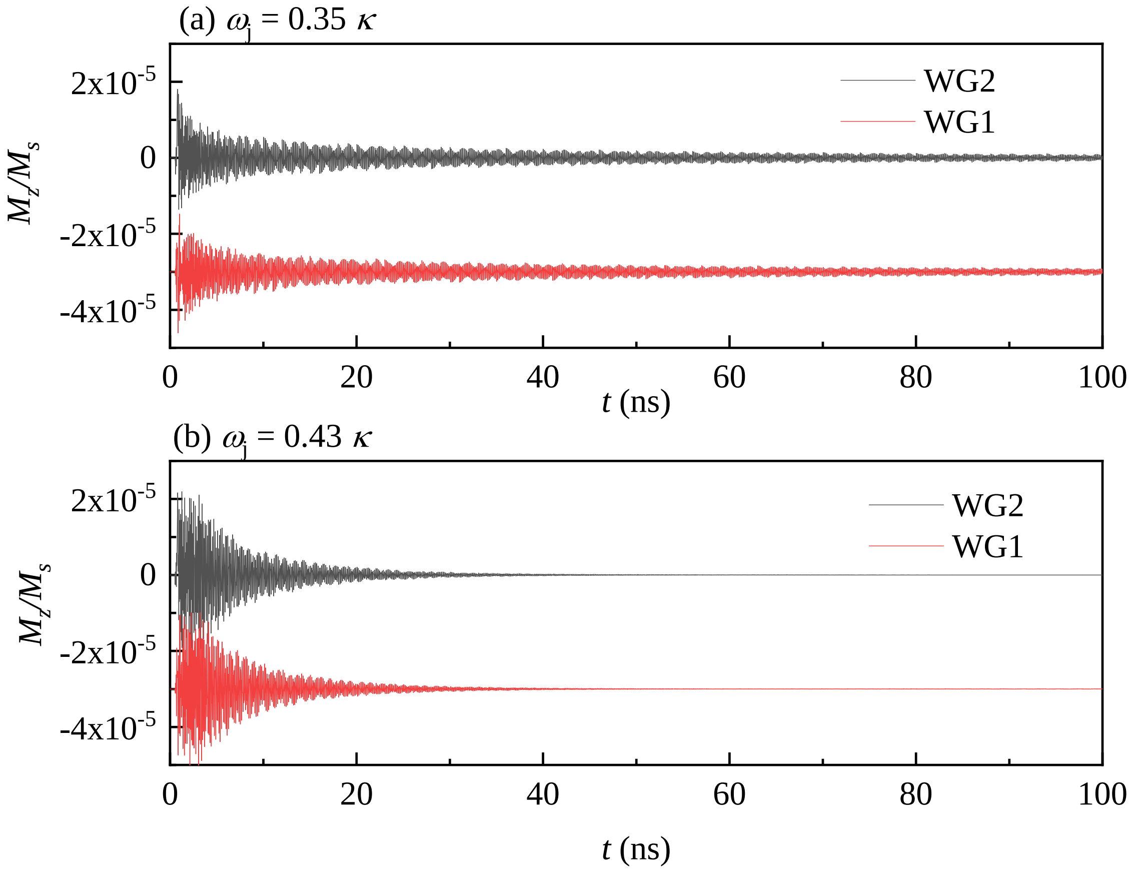


FIG. S5. For the periodic SOT frequency $\omega_{\mathrm{J,t}}$ (with amplitude $\omega_{\mathrm{J}}$), when (a) $\omega_{\mathrm{J}}/\kappa = 0.35$ and (b) $\omega_{\mathrm{J}}/\kappa = 0.43$ (outside the instability range), time-dependent $M_{\mathrm{z}}$ at $x = 2000$ nm in WG1 and WG2 (obtained from the micromagnetic simulation based on the LLG equation). The red curves (WG1) are in the same range with WG2 curves, which are intentionally offset for clarity.

and expanding the eigenfunctions with respect to a suitable basis incorporating the periodic conditions, we obtain the eigenvalues for different bands folded into the first BZ, as shown in Fig. S7. Due to the periodically varying exchange coupling, magnon band gaps are found at $k_{\mathrm{x}} = 0$. Comparing with the cases under amplitude $\omega_{\mathrm{J0}} = 0$ and $\omega_{\mathrm{J0}} = 0.1\kappa$, we find the effect of spatially-periodic SOT $\omega_{\mathrm{J}}(x)$ is especially dominant when two magnon modes approach each other at $k/k_{\mathrm{J}} = 0.51$. Here, $\omega_{\mathrm{J}}(x)$ enlarges the crossing area with collapsed real components, and in the same range the imaginary components are clearly separated. These features indicate the range is above EP. It is also found that EP is dependent on the wave-vector $k$, as demonstrated by Fig. S8. In particular, near the crossing point ($k/k_{\mathrm{J}} = 0.51$), the two modes collapse at the EP near $\omega_{\mathrm{J0}} = 0$. Away from the cross point,

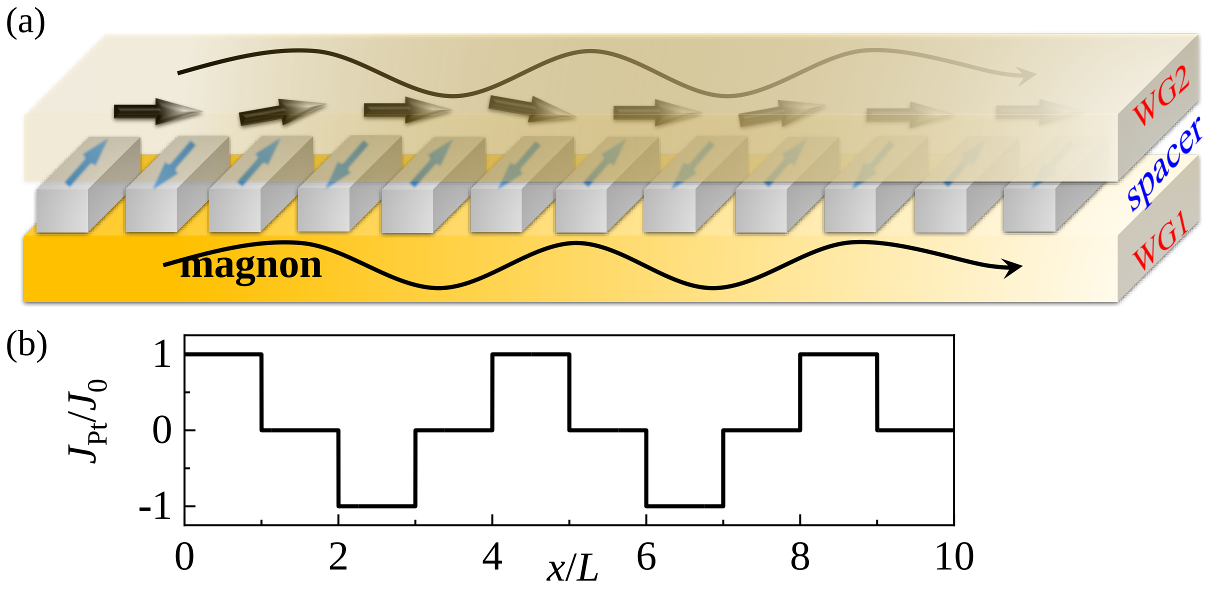


FIG. S6. (a) The magnetic films are periodically RKKY-coupled at the Pt stripes region, resulting in a magnonic crystal. The system is periodic PT symmetric: The charge current-carrying Pt stripes are periodically separated by a distance $L$ along $x$ and have a width $L$ along $x$, resulting in a gain/loss grating for the magnonic crystal. (b) The space period current $J_{\rm Pt}$ with period $4L$ used in the simulations.

the $\omega_{\rm J0}$ amplitude at EP becomes larger, see the case at $k/k_{\rm J} = 0.3$. Above the EP, when one imaginary component turns positive, the self-sustaining auto-oscillation can be driven effectively (Fig. S9).

In Fig. S8(b), one imaginary component turns positive indicating the amplified SW. As proved by numerical simulations (Fig. S9), the spin wave is amplified with time, and mainly the frequency at the cross point is excited (see the spectra in Figs. S9(c) and (f)). We note for a large enough amplitude, a strong nonlinear oscillation causes instability (Fig. S9(d-f)), but the oscillation is still mainly distributed at the crossed frequency at $k/k_{\rm J} = 0.51$.

## IV. MAGNONICS WITH SPATIALLY-PERIODIC LOSS/MORE-LOSS MECHANISM

In the main text, the EPs are generated in the system subjected to coupled gain and loss. Here, we analyze the EP generated via coupled loss and periodic more-loss. Such

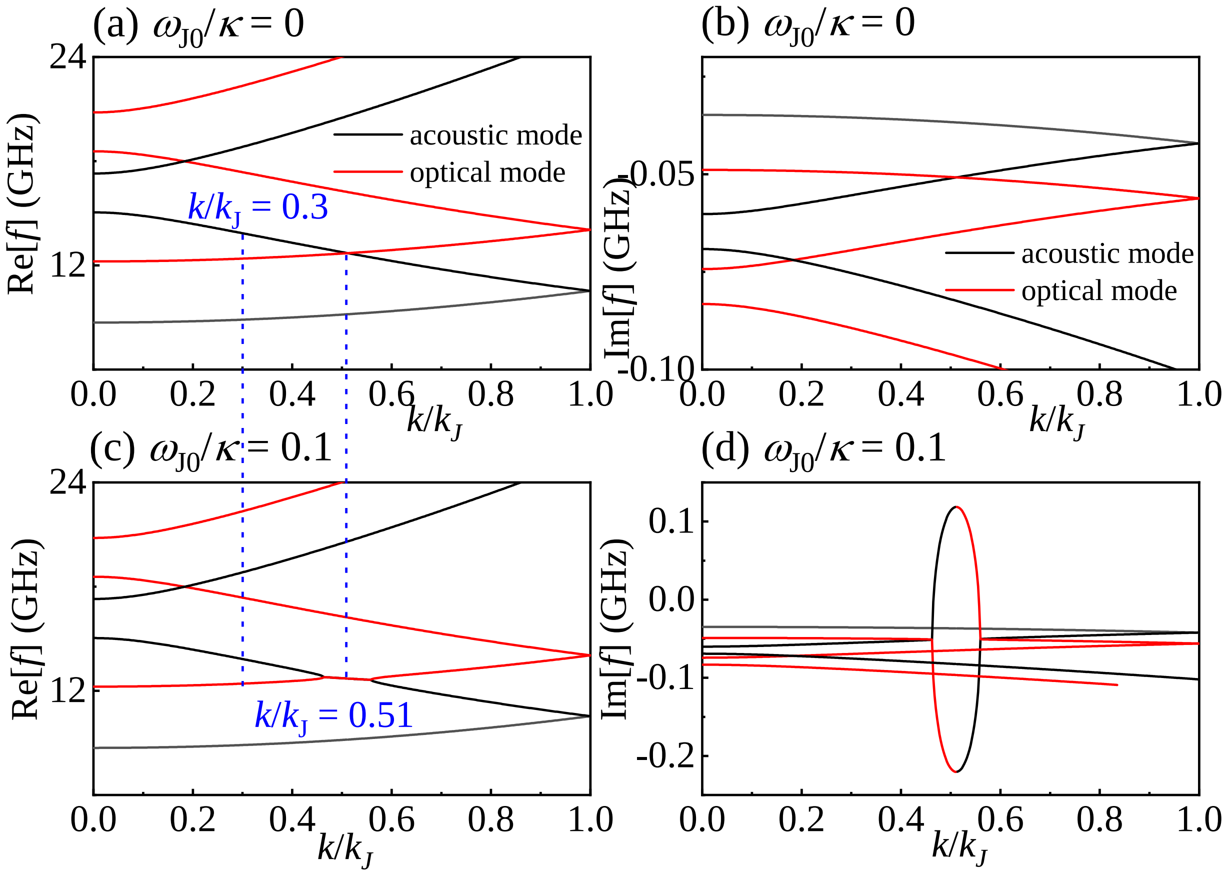


FIG. S7. For the model of Fig. S6(a), the real (dispersion) and the imaginary components of magnon eigenfrequencies folded at the BZ boundaries $k = 0$ and $k_{\rm J}$ (a-b) without spatial amplitude ($\omega_{\rm J0} = 0$) and (c-d) with ($\frac{\omega_{\rm J0}}{\kappa} = 0.1$) the spatially varying electric current density. Here, the period of electric current is $4L = 80$ nm and $k_{\rm J} = \frac{\pi}{4L}$.

situation is realized by optical grating generated by laser beams in one (WG1) of two coupled waveguides. A focused laser can enhance locally the losses, and so an optical grating results in the spatially-periodic damping $\alpha$ in WG1.[3] Here, we use the form $\alpha = \alpha_0 + \alpha_1 \cos^2(k_\alpha x)$ in WG1, while in WG2 $\alpha = \alpha_0$. With the Bloch theorem we obtain the numerical eigenvalues folded at the BZ boundaries, as shown in Fig. S10. We find that the coupled loss and more-loss still can bring about qualitatively the features of the EP. Near the cross point $\frac{k}{k_\alpha} = 0.63$, the range above the EP is identified. Moreover, at a fixed $k$, we find that at the EP (or EP adjacent) two real components are very close, and two imaginary components start to separate. Further increasing $\alpha_1$, the increase in differences between imaginary components is much larger than for the real components, signaling phenomena typical for above EP regime.

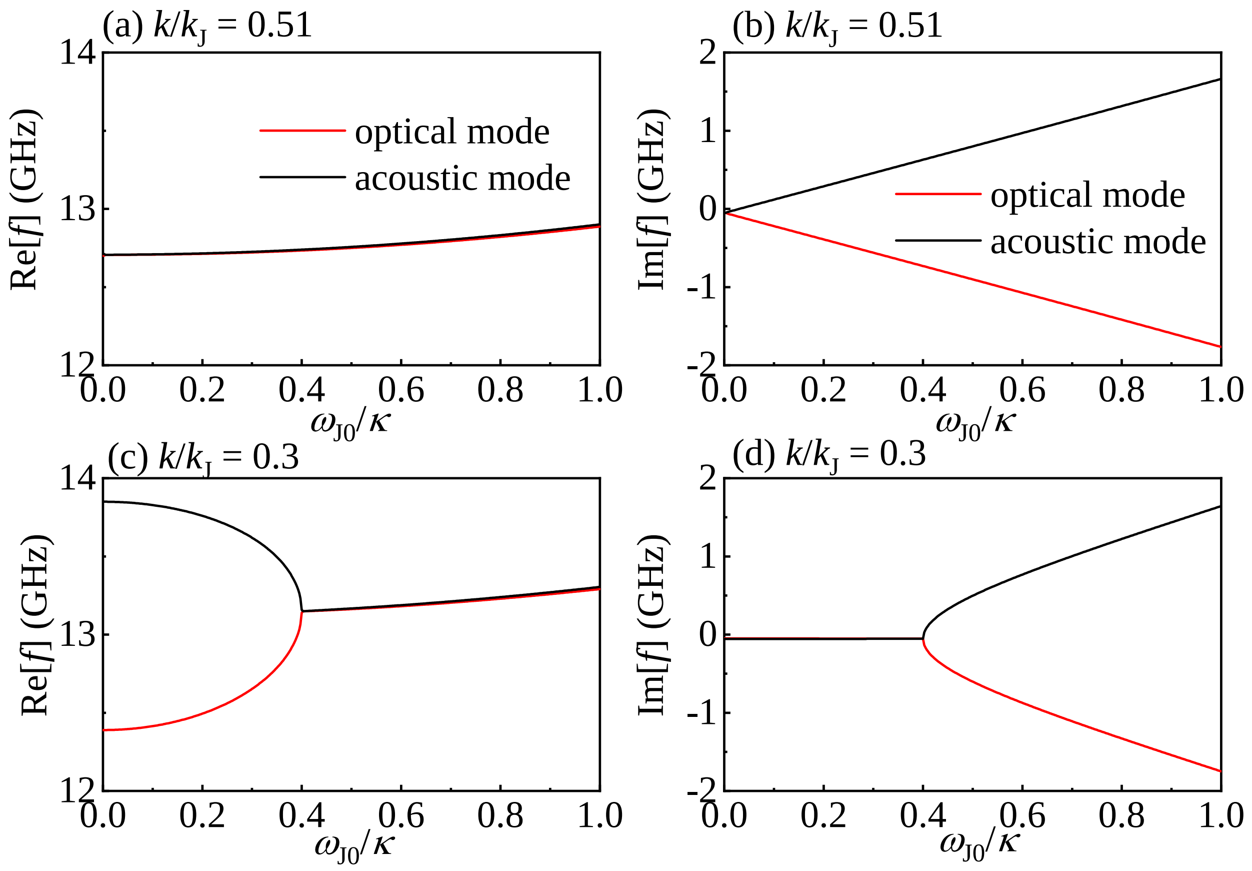


FIG. S8. At $\frac{k}{k_{\rm J}}$ = (a-b) 0.51 and (c-d) 0.3, real (dispersion) and imaginary components of magnon eigenfrequencies as functions of electric current density amplitude $\omega_{\rm J0}$. Here, the spatial period of electric current is $4L = 80$ nm and $k_{\rm J} = \frac{\pi}{4L}$.

In addition, different from gain/loss, here in range near the BZ boundary $k = k_\alpha$, we also find the features above the EP in Fig.S10(a-b), where two magnon modes are interacting with themselves separately.

## V. INFLUENCE OF THE DIPOLE-DIPOLE INTERACTION

In this section, we consider the role of the dipole-dipole interaction in the Floquet model. We find the dipole-dipole interaction only slightly affects the values of quasienergies and quasi-EPs. The main conclusions concerning the Floquet broken PT-symmetry phase and auto-oscillation remain unaltered. We note the following model was adopted for describing the PT-symmetry with constant electric current in Ref. [4]. The dipolar interaction provides additional coupling between magnons of different waveguides, and slightly increases the

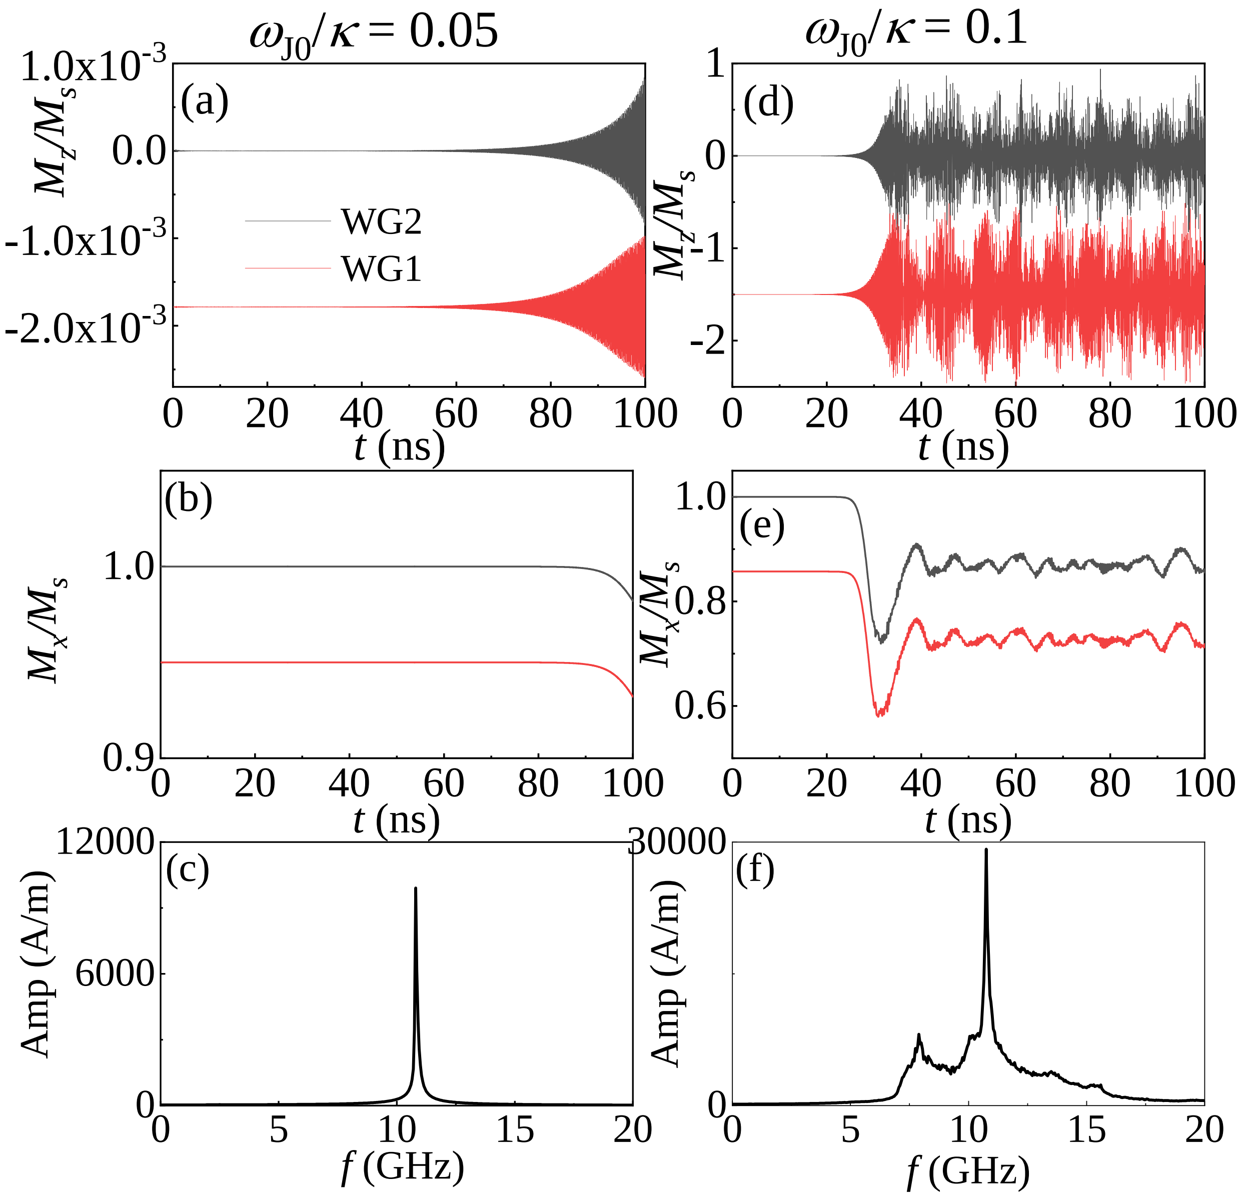


FIG. S9. Under $\frac{\omega_{J0}}{\kappa}$ = (a-c) 0.05 and (d-f) 0.1, time-dependent (a,d) $M_z(x = 2000\text{nm})$ and (b,e) averaged $M_x$ in WG1 and WG2. (c) and (f) are frequency spectra of magnetization oscillations in last 20 ns. Spin waves are triggered by the sinc pulse $h(t) = h_a\mathbf{z}\sin(2\pi f_H t)/(2\pi f_H t)$ with amplitude $h_a = 1 \times 10^5$ A/m and frequency range $f_H = 50$ GHz, applied to the region at $x = 0$. The red curves (WG1) are in the same range with WG2 curves, which are intentionally offset for clarity.

value of EP. Comparing the case without the dipolar coupling, the PT-symmetry related phenomena still exist.

Here we adopt a similar model from the main text. Two stripe waveguides are coupled

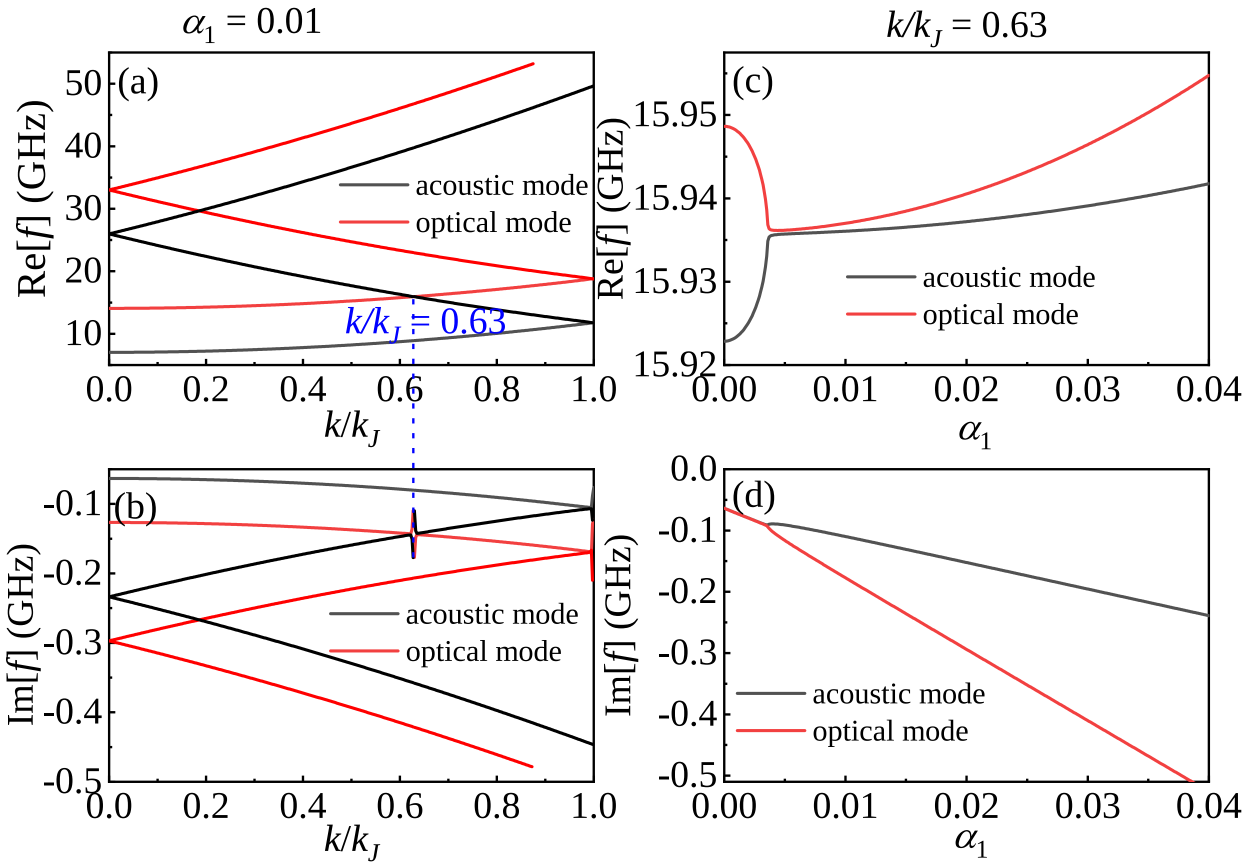


FIG. S10. (a-b) With the grating induced periodic damping $\alpha = \alpha_0 + \alpha_1 \cos^2(k_\alpha x)$ in WG1. real (dispersion) and imaginary components of magnon eigenfrequencies folded at the BZ boundaries $k = 0$ and $k_\alpha$. Here, $\alpha_0 = 0.004$, $\alpha_1 = 0.01$, and $k_\alpha = 0.06\ \mathrm{nm}^{-1}$. (c-d) At $\frac{k}{k_\alpha} = 0.63$, real (dispersion) and imaginary components of magnon eigenfrequencies as functions of $\alpha_1$.

via the RKKY interaction and the dipole-dipole interaction across the non-magnetic spacer. The thickness (along $z$ axis) of waveguides is $t = 4$ nm, and gap between the waveguides is $\sigma = 4$ nm. The magnetization vectors with small derivations in the two waveguides ($p = 1, 2$) are expressed in the form of $\mathbf{m}_{\mathrm{p}}(r,t) = \mathbf{m}_{0,\mathrm{p}} + \mathbf{m}_{\mathrm{s,p}} e^{i(\mathbf{k}_{\mathrm{s}}\cdot\mathbf{r}-\omega t)}$. Here, $\mathbf{m}_{0,\mathrm{p}} = \mathbf{y}$ is the static equilibrium magnetization parallel to $y$ axis, and the small deviation from the equilibrium is $\mathbf{m}_{\mathrm{s,p}} = (\delta m_{\mathrm{x,p}}, 0, \delta m_{\mathrm{z,p}})$ with $\delta m_{\mathrm{x(z),p}} \ll 1$. The wave vector $\mathbf{k}_{\mathrm{s}}$ is the sum of the in-plane wave vector $\mathbf{k} = k_{\mathrm{x}}\mathbf{x} + k_{\mathrm{y}}\mathbf{y}$ and the perpendicular (to the $x$-$y$ plane) wave vector $k_{\mathrm{z}}$. Then, with the Fourier representation of the linearized LLG equation, we derive

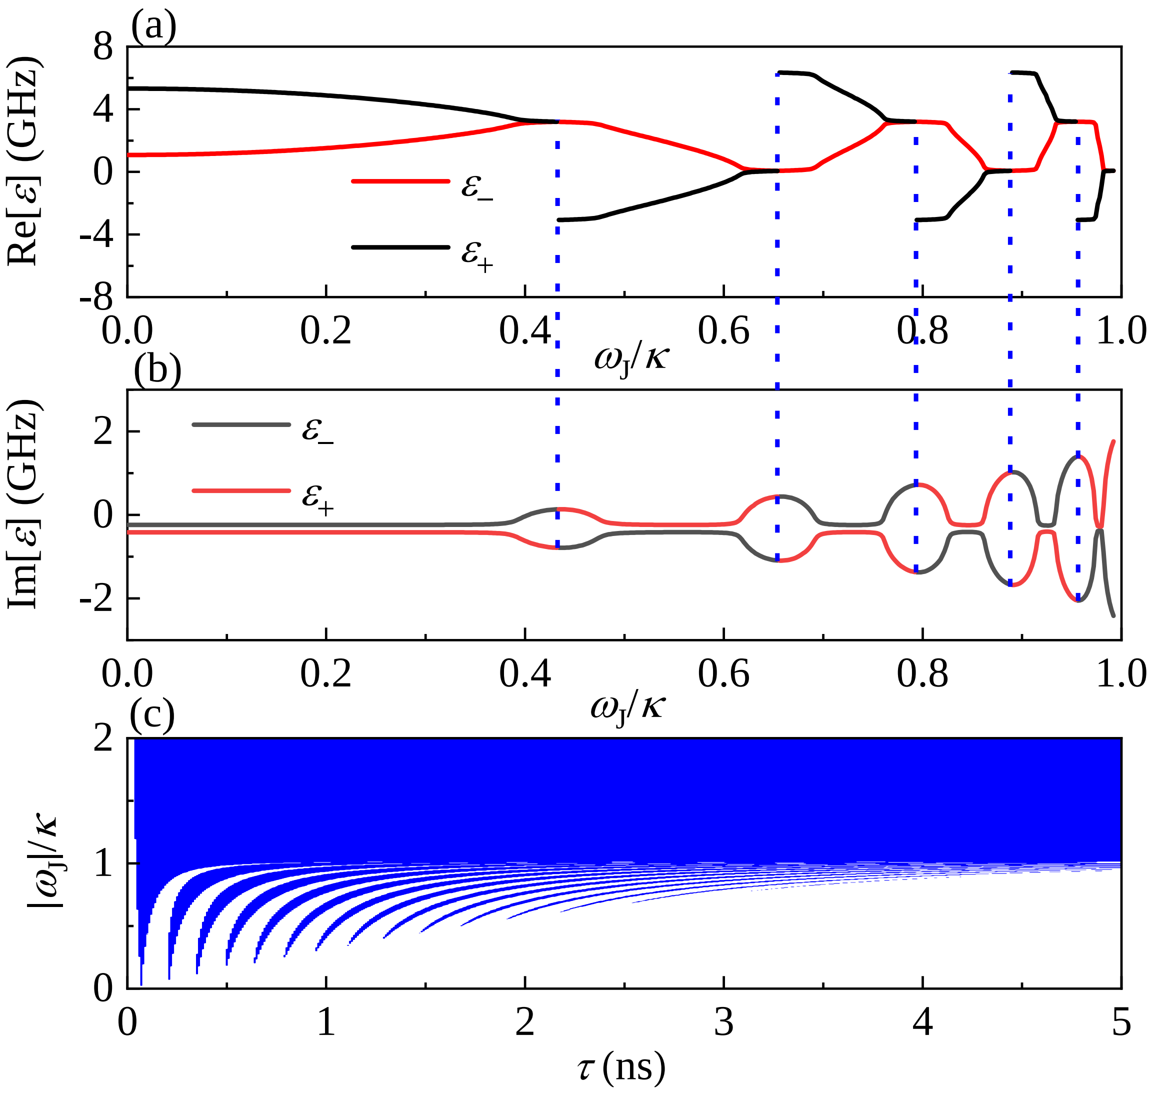


FIG. S11. For the periodic SOT $\omega_{\rm J,t}$ (with amplitude $\omega_{\rm J}$) applied to the coupled waveguides with dipolar interaction, (a) real and (b) imaginary parts of quasienergies $\epsilon_{\pm}$ as functions of the amplitude $\omega_{\rm J}$ with the period parameter $\tau = 1$ ns and $k_{\rm x} = 0$. (c) The stability phase diagram on the $\tau - \omega_{\rm J}$ space with $k_{\rm x} = 0$. The shaded region corresponds to the unstable oscillation.

the following expression for the spin wave,

$$-i\omega \mathbf{m}_{\rm s,p} = \mathbf{m}_{\rm 0,p} \times \sum_{\rm q} \hat{\Omega}_{\rm pq} \cdot m_{\rm s,q} - \mathbf{m}_{\rm 0,p} \times (i\alpha\omega \mathbf{m}_{\rm s,p} - \omega_{\rm J} \mathbf{T}_{\rm p} \times \mathbf{m}_{\rm s,p}). \tag{S1}$$

$p, q = 1, 2$ enumerates the two waveguides, and the tensor $\hat{\Omega}_{\rm pq}$ has the form,

$$\hat{\Omega}_{\rm pq} = \omega_0 \delta_{\rm pq} \hat{I} + \omega_{\rm M} \hat{F}(d_{\rm pq}) + \kappa(\delta_{\rm pq} - 1)\hat{I}. \tag{S2}$$

Here, we introduce $\omega_0 = \gamma H_0 + \frac{2\gamma A_{\rm ex} k^2}{\mu_0 M_{\rm s}} + \kappa$, $\kappa = \gamma \frac{J_{\rm RKKY}}{\mu_0 M_{\rm s} t_{\rm p}}$, and $\omega_{\rm M} = \gamma M_{\rm s}$. The wave

vector $k$ is equal to $\sqrt{k_\mathrm{x}^2+k_\mathrm{y}^2}$, the distance between the two waveguides $d_{12}=t+\sigma$, $t$ is the waveguide thickness, and $\sigma$ is the gap between the waveguides. The dynamic magnetodipolar interaction is described by the tensor $\hat{\mathbf{F}}$ [5–8]:

$$\begin{aligned}\hat{F}(d_\mathrm{pq}) &= \int \hat{N}(d_\mathrm{pq})e^{i\mathbf{k}\cdot\mathbf{r}}\frac{d^2\mathbf{k}}{(2\pi)^2},\\ \mathbf{N}^{\alpha\beta}(d_\mathrm{pq}) &= \frac{1}{t}\int D_\mathrm{p}(k_\mathrm{z})D^*_\mathrm{q}(k_\mathrm{z})\frac{k_\alpha k_\beta}{k^2}e^{ik_\mathrm{z}d_\mathrm{pq}}\frac{dk_\mathrm{z}}{2\pi}.\end{aligned} \tag{S3}$$

The "shape amplitude" $D_\mathrm{p}(k_\mathrm{z})=\int_0^t m(z)e^{-ik_\mathrm{z}z}dz$ describes the influence of the finite thickness $t$ of the thin waveguide. The width profile of the SW mode in the waveguide is usually nonuniform ($m(z)\sim\cos(k_\mathrm{z}^p z)$) due to the pinning effect from the geometric boundaries. For the thickness of the waveguide close to or smaller than the material exchange length or the free effective boundary condition, the SW profile is almost uniform, i.e., $m(z)=1$. By setting $\psi_\mathrm{p}^\pm=\delta m_\mathrm{x,p}\pm i\delta m_\mathrm{z,p}$, we obtain the spin wave equation,

$$\begin{aligned}
&i\frac{\partial\psi_1^+}{\partial t}-(\omega_1^+-i\omega_\mathrm{J}^+)\psi_1^+-(\omega_\mathrm{x}^+-\omega_\mathrm{z}^+)\psi_1^--(\omega_\mathrm{x,d}^++\omega_\mathrm{z,d}^+-\kappa^+)\psi_2^+-(\omega_\mathrm{x,d}^+-\omega_\mathrm{z,d}^+)\psi_2^-=0,\\
&i\frac{\partial\psi_1^-}{\partial t}+(\omega_\mathrm{x}^--\omega_\mathrm{z}^-)\psi_1^++(\omega_1^-+i\omega_\mathrm{J}^-)\psi_1^-+(\omega_\mathrm{x,d}^--\omega_\mathrm{z,d}^-)\psi_2^++(\omega_\mathrm{x,d}^-+\omega_\mathrm{z,d}^--\kappa^-)\psi_2^-=0,\\
&i\frac{\partial\psi_2^+}{\partial t}-(\omega_\mathrm{x,d}^++\omega_\mathrm{z,d}^+-\kappa^+)\psi_1^+-(\omega_\mathrm{x,d}^+-\omega_\mathrm{z,d}^+)\psi_1^--(\omega_1^++i\omega_\mathrm{J}^+)\psi_2^+-(\omega_\mathrm{x}^+-\omega_\mathrm{z}^+)\psi_2^-=0,\\
&i\frac{\partial\psi_2^-}{\partial t}+(\omega_\mathrm{x,d}^--\omega_\mathrm{z,d}^-)\psi_1^++(\omega_\mathrm{x,d}^-+\omega_\mathrm{z,d}^--\kappa^-)\psi_1^-+(\omega_\mathrm{x}^--\omega_\mathrm{z}^-)\psi_2^++(\omega_1^--i\omega_\mathrm{J}^-)\psi_2^-=0.
\end{aligned} \tag{S4}$$

We introduced the following notions $\omega_1=\omega_0+\omega_\mathrm{M}F^{xx}(0)/2+\omega_\mathrm{M}F^{zz}(0)/2$, $\omega_\mathrm{x}=\omega_\mathrm{M}F^{xx}(0)/2$, $\omega_\mathrm{z}=\omega_\mathrm{M}F^{zz}(0)/2$, $\omega_\mathrm{x,d}=\omega_\mathrm{M}F^{xx}(d_{12})/2$, $\omega_\mathrm{z,d}=\omega_\mathrm{M}F^{zz}(d_{12})/2$, $\omega_1^\pm=\omega/(1\pm i\alpha)$, $\omega_\mathrm{x(z),d}^\pm=\omega_\mathrm{x(z),d}/(1\pm i\alpha)$, $\omega_\mathrm{J}^\pm=\omega_\mathrm{J,t}/(1\pm i\alpha)$ and $\kappa^\pm=\kappa/(1\pm i\alpha)$. Then, solving the above equations and obtaining the periodic evolution matrix, with the Floquet's theorem we numerically derivate the quasienergies $\epsilon_\pm$ as shown in Fig. S11. Here, same material prameters are adopted in the numerical calculation, and we use a larger damping constant $\alpha=0.004$.

For the Floquet time periodic PT symmetry, the dipolar interaction slightly changes the values of quasi-EPs. For example, in the main text the imaginary parts are more separated between $0.34\kappa\leq\omega_\mathrm{J}\leq 0.43\kappa$, and the dipolar interaction changes this to $0.39\kappa\leq\omega_\mathrm{J}\leq 0.48\kappa$. Other quasi-EPs and PT-symmetry broken regions are also slightly shifted. We also identify the similar stability phase diagram in Fig. S11(c). The instability islands in this case are slightly shifted by the dipolar interaction. For example, at $\tau=7\times10^{-11}$ s, the smallest SOT frequency amplitude $\omega_\mathrm{J}$ changes from $0.032\kappa$ to $0.048\kappa$.

## REFERENCES


[1] D. Houssameddine, U. Ebels, B. Delaët, B. Rodmacq, I. Firastrau, F. Ponthenier, M. Brunet, C. Thirion, J.-P. Michel, L. Prejbeanu-Buda, M.-C. Cyrille, O. Redon, and B. Dieny, Spin-torque oscillator using a perpendicular polarizer and a planar free layer, Nature Mater. **6**, 447 (2007).

[2] S. Kaka, M. R. Pufall, W. H. Rippard, T. J. Silva, S. E. Russek, and J. A. Katine, Mutual phase-locking of microwave spin torque nano-oscillators, Nature **437**, 389 (2005).

[3] A. V. Sadovnikov, A. A. Zyablovsky, A. V. Dorofeenko, and S. A. Nikitov, Exceptional-point phase transition in coupled magnonic waveguides, Phys. Rev. Appl. **18**, 024073 (2022).

[4] X.-g. Wang, G.-h. Guo, and J. Berakdar, Steering magnonic dynamics and permeability at exceptional points in a parity–time symmetric waveguide, Nat. Commun. **11**, 5663 (2020).

[5] Q. Wang, P. Pirro, R. Verba, A. Slavin, B. Hillebrands, and A. V. Chumak, Reconfigurable nanoscale spin-wave directional coupler, Sci. Adv. **4**, e1701517 (2018).

[6] R. Verba, G. Melkov, V. Tiberkevich, and A. Slavin, Collective spin-wave excitations in a two-dimensional array of coupled magnetic nanodots, Phys. Rev. B **85**, 014427 (2012).

[7] M. Beleggia, S. Tandon, Y. Zhu, and M. D. Graef, On the magnetostatic interactions between nanoparticles of arbitrary shape, J. Magn. Magn. Mater. **278**, 270 (2004).

[8] X.-g. Wang, L. Chotorlishvili, G.-h. Guo, and J. Berakdar, High-fidelity magnonic gates for surface spin waves, Phys. Rev. Applied **12**, 034015 (2019).
